# Supplementary material for: Convergence of a Relaxed Variable Splitting Method for Learning Sparse Neural Networks via $\ell_1, \ell_0$, and transformed-$\ell_1$ Penalties
Source: arXiv:1812.05719 source file (2020-02-25)
Supplement: Supplementary file 1 [file Appendix.tex]

\documentclass{article}
\usepackage{amsmath,amsthm,amssymb,dsfont,mathtools,bbm,bm}
\usepackage{booktabs}
\usepackage[table]{xcolor}
\usepackage{float}
\usepackage[ruled,vlined]{algorithm2e}
\usepackage[utf8]{inputenc} % allow utf-8 input
\usepackage[T1]{fontenc}    % use 8-bit T1 fonts
\usepackage{url}            % simple URL typesetting
\usepackage{booktabs}       % professional-quality tables
\usepackage{amsfonts}       % blackboard math symbols
\usepackage{nicefrac}       % compact symbols for 1/2, etc.
\usepackage{microtype}      % microtypography

\theoremstyle{definition}

\begin{document}

\end{document}
